# Supplementary material for: RHH-LGP: Receding Horizon And Heuristics-Based Logic-Geometric Programming For Task And Motion Planning
Source: arXiv:2110.03420 source file (2022-03-06)
Supplement: Supplementary file 1 [file appendix.tex]

\subsection{Additional results}
\begin{table}[htbp]
\centering
\begin{tabular} {@{}rrrrr@{}} \toprule
$n$ & Time in s. & \# Tree nodes & \# Expanded & Sol. len. \\
\midrule
1       & 11.81     & 576       & 77        & 11 \\
2       & 111.39    & 1197      & 153       & 14 \\
4       & 151.42    & 1375      & 145       & 12 \\
8       & 30.90     & 1157      & 77        & 12 \\
\bottomrule
\end{tabular}
\caption{Climbing task with multiple goals planned with MBTS + action-specific heuristics.}\label{tbl:complex}
\end{table}
\begin{table*}[htbp]
\centering
\resizebox{\linewidth}{!}{%
\begin{tabular} {@{}rrrrrcrrrr@{}} \toprule
\multicolumn{1}{c}{$n$} & \multicolumn{4}{c}{One crawler} & \phantom{abc} & \multicolumn{4}{c}{Two crawlers} \\
\cmidrule{2-5} \cmidrule{7-10} & Time in s. & \# Tree nodes & \# Expanded & Sol. len. && Time in s. & \# Tree nodes & \# Expanded & Sol. len. \\
\midrule
1       & 0.08      & 10        & 2         & 2  && 0.48        & 21      & 3         & 2 \\
2       & 0.56      & 49        & 11        & 5  && 7.00        & 81      & 13        & 2 \\
4       & 2.69      & 85        & 13        & 7  && 13.59       & 190     & 22        & 8 \\
8       & 3.61      & 181       & 17        & 10 && 11.64       & 309     & 23        & 9 \\
16      & 22.41     & 505       & 27        & 16 && 16.38       & 590     & 26        & 11 \\
32      & 444.26    & 5849      & 171       & 50 && 138.03      & 2066    & 47        & 19 \\
64      & --        & --        & --        & -- && 439.01      & 4088    & 53        & 27 \\
\bottomrule
\multicolumn{10}{l}{\footnotesize Note: scenarios without metrics could not be solved at all}\\
\end{tabular}}
\caption{Planning the climbing task using MBTS and action-specific heuristics for different numbers of available modules.}\label{tbl:exp3}
\end{table*}
\begin{table}[htbp]
\centering
\begin{tabular} {@{}rrrrr@{}} \toprule
$n$ & Time in s. & Tree nodes & Expanded nodes & Solution len. \\
\midrule
1       & 1.84      & 7        & 2      & 3  \\
2       & 2.18      & 12       & 4      & 5  \\
4       & 3.45      & 25       & 8      & 9 \\
8       & 17.40     & 63       & 16     & 17 \\
\bottomrule
\end{tabular}
\caption{Modular robot pick-and-place task planned with MBTS and action-specific heuristics.}\label{tbl:exp4}
\end{table}
